# Supplementary material for: Breaking the Convergence Barrier: Optimization via Fixed-Time Convergent Flows
Source: arXiv:2112.01363 source file (2022-03-20)
Supplement: Supplementary file 1 [file SupportingInfo.pdf]

# Tuning Adam on MNIST

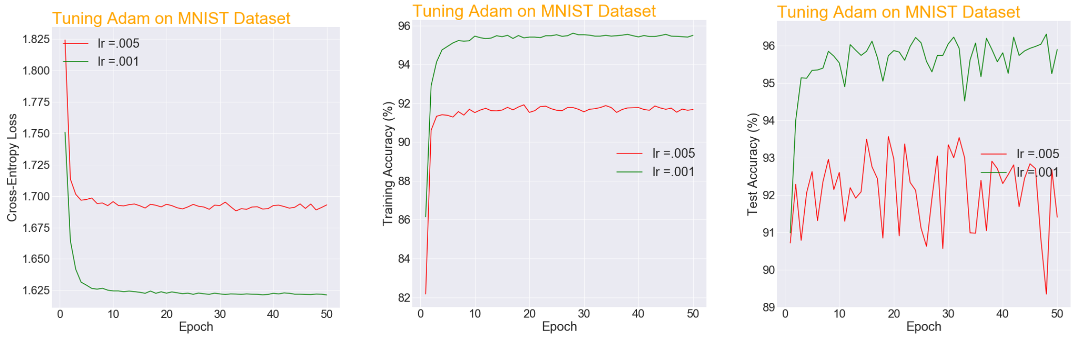


(a) (b) (c)

Figure 1: Tuning Adam on MNIST. (a) Cross-entropy training loss, (b) Training accuracy, (c) Testing Accuracy. It can be seen that Adam with a learning rate of 0.005 does not work as well as with a learning rate of 0.001.

# Snapshots of Minimization of Rosenbrock Function

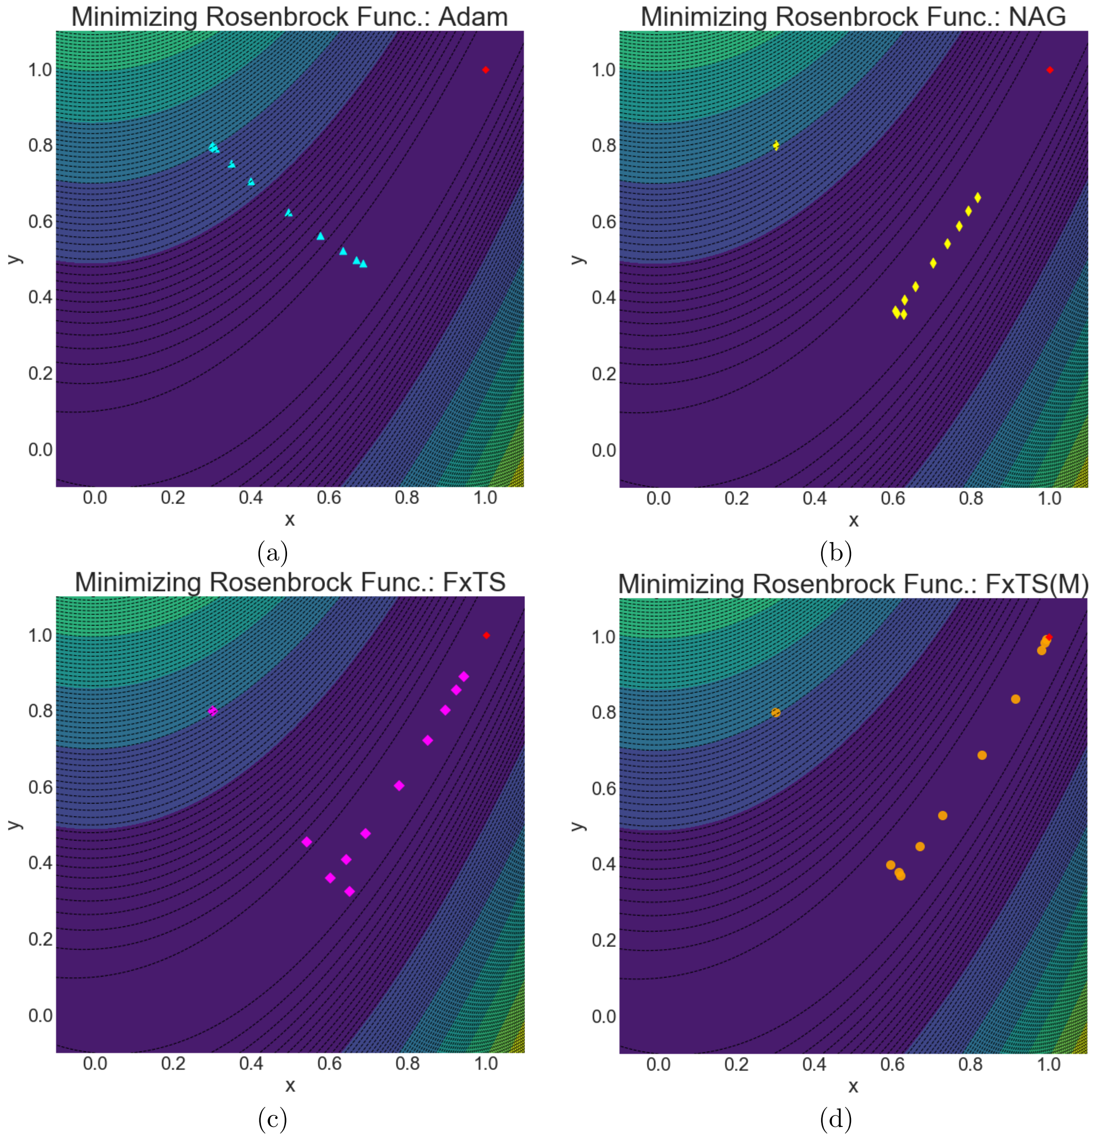


Figure 2: Minimization of Rosenbrock function. Snapshots of trajectories of various optimization algorithms at epochs 1, 4, 7, 10, 50, 100, 200, 300, 400, 500, 600 for the initial condition $(0.3, 0.8)$. (a) Adam (b) Nesterov Accelerated Gradient (c) FxTS-GF (d) FxTS(M)-GF.

## Minimization of Beale function

Figure 3b depicts evolution of trajectories of various optimization algorithms starting at the initial condition $(-2, 2)$. The Beale function is shown in Figure 3a. It has a global minimum at $(3, 0.5)$. The hyperparameters of the various optimization algorithms were chosen as:
**Adam**: Learning rate $= 10^{-3}$
**NAG**: Learning rate $= 10^{-4}$, Momentum $= 0.1$. NAG with a learning rate of $10^{-3}$ or with higher-momentum turned out to be unstable.
**FxTS-GF**: Learning rate $= 10^{-3}$, $\alpha$'s=(2.5,1.8), $\beta$'s=(1.25,1.25)
**FxTS(M)-GF**: Learning rate $= 10^{-3}$, $\alpha$'s=(2.5,1.8), $\beta$'s=(1.25,1.25), Momentum $= 0.01$

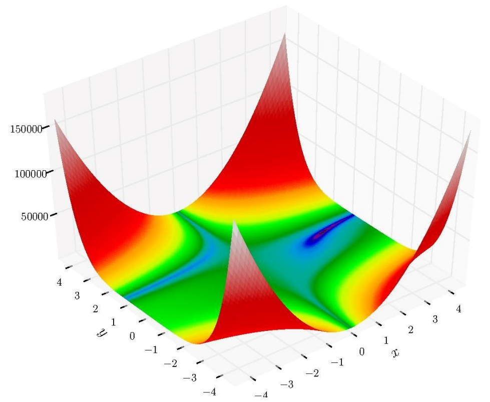

(a)

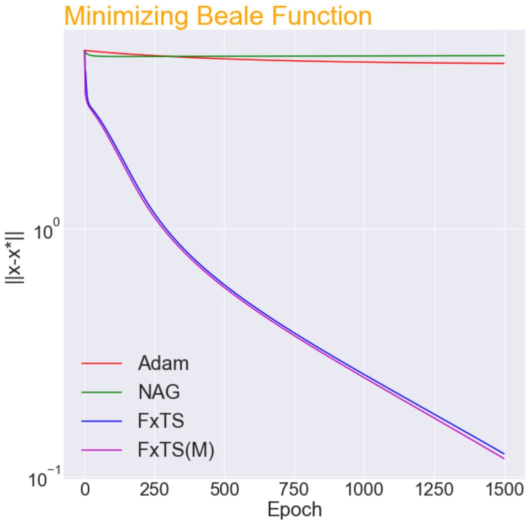


(b)

$$f(x, y) = (1.5 - x + xy)^2 + (2.25 - x + xy^2)^2 + (2.625 - x + xy^3)^2$$

$$(x^\star, y^\star) = (3, 0.5)$$

Figure 3: Minimization of Beale function for the initial condition $(-2, 2)$. (a) Function definition. (b) Comparison of various optimization algorithms.

## Minimization of McCormick function

Figure 4b depicts evolution of trajectories of various optimization algorithms starting at the initial condition $(-1.2, 2)$. The McCormick function is shown in Figure 4a. It has a global minimum at $(-0.54719, -1.54719)$. The hyperparameters of the various optimization algorithms were chosen as:

**Adam**: Learning rate $= 10^{-3}$

**NAG**: Learning rate $= 10^{-3}$, Momentum $= 0.5$

**FxTS-GF**: Learning rate $= 10^{-3}$, $\alpha$'s=(20,1.98), $\beta$'s=(1.25,1.25)

**FxTS(M)-GF**: Learning rate $= 10^{-3}$, $\alpha$'s=(20,1.98), $\beta$'s=(1.25,1.25), Momentum $= 0.1$

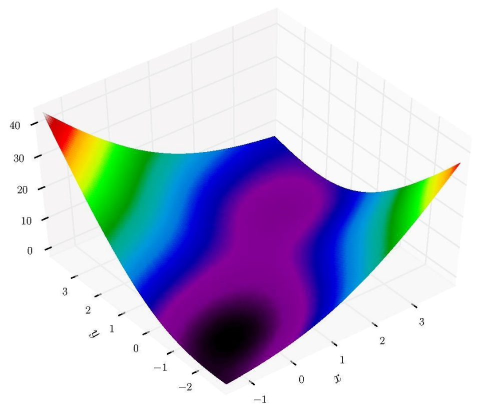


(a)

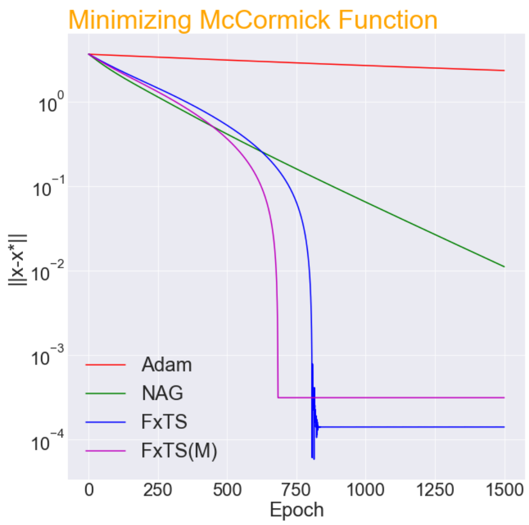


(b)

$f(x, y) = \sin(x + y) + (x - y)^2 - 1.5x + 2.5y + 1$ $\qquad$ $(x^\star, y^\star) = (-0.54719, -1.54719)$

Figure 4: Minimization of McCormick function for the initial condition $(-1.2, 2)$. (a) Function definition. (b) Comparison of various optimization algorithms.

## Additional visualizations and code

We also compared various optimization algorithms for minimization of Rosenbrock function at varying initial conditions. FxTS-GF and FxTS(M)-GF were found to converge to the minimizer much faster than Adam and NAG methods. Videos of evolution of trajectories for different initial conditions are included in the supplementary material, along with the accompanying codes.

## PyTorch implementation of FxTS(M)-GF

```
import torch
from torch.optim import Optimizer

class FxTS_momentum(Optimizer):
    """ Implements FxTS optimizer with momentum
    Parameters:
        lr (float): learning rate. Default 1e-3
        betas (tuple of two floats): FxTS beta parameters (b1,b2). Default: (0.9,0.9)
        alphas (tuple of two floats): FxTS alpha parameters (a1,a2). Default: (2.1,1.9)
    """
    def __init__(self,params,lr=1e-3, betas=(0.9,0.9),alphas=(2.1,1.9),momentum = 0.0):
        if lr < 0.0:
            raise ValueError("Invalid learning rate:{}-should be >= 0.0".format(lr))
        if betas[0] < 0.0:
            raise ValueError("Invalid beta param:{}-should be >= 0.0".format(betas[0]))
        if betas[1] < 0.0:
            raise ValueError("Invalid beta param:{}-should be >= 0.0".format(betas[1]))
        if not alphas[0] > 2.0:
            raise ValueError("Invalid alpha param:{}-should be > 2.0".format(alphas[0]))
        if not 1.0 < alphas[1] < 2.0:
            raise ValueError("Invalid alpha param:{}-should be >1., <2.".format(alphas[1]))
        if not 0.0 <= momentum < 1.0:
            raise ValueError("Invalid momentum param:{}-should be >=0., <1.".format(momentum))

        defaults = dict(lr=lr, betas=betas, alphas=alphas, momentum=momentum)
        super(FxTS_momentum, self).__init__(params, defaults)

    def __setstate__(self, state):
        super(FxTS_momentum, self).__setstate__(state)

    def step(self, closure=None):
        """ Performs a single optimization step.
        Arguments:
            closure (callable, optional): A closure that reevaluates the model
                and returns the loss.
        """
        loss = None
        if closure is not None:
            loss = closure()

        for group in self.param_groups:
            beta1, beta2   = group['betas']
            alpha1, alpha2 = group['alphas']
            lr             = group['lr']
            momentum       = group['momentum']
```

```
        for p in group['params']:
            if p.grad is None:
                continue

            grad      = p.grad.data

            state = self.state[p]
            if len(state) == 0:
                state['step'] = 0
                # Exponential moving average of gradient values
                state['v'] = torch.zeros_like(p.data)

            v = state['v']
            state['step'] += 1
            v.mul_(momentum).add_((1-momentum),grad)

            v_norm = v.norm()
            factor = beta1/(v_norm ** ((alpha1-2)/(alpha1-1))) + \
                     beta2/(v_norm ** ((alpha2-2)/(alpha2-1)))
            v.mul_(factor)

            if  grad.norm() > (grad-v).norm():
                h = 0.2/(grad.norm() ** ((alpha1-2)/(alpha1-1))) + \
                    0.2/(grad.norm() ** ((alpha2-2)/(alpha2-1)))
            else:
                h = 1.

            p.data.add_(-h*lr,v)

    return loss
```

In practice, $h(x, v) \equiv 1$ also yields very similar results and FxTS-GF(M) can instead be implemented with $h(x, v) = 1$ for the sake of simplicity. The factor of 0.2 in the definition of $h(x, v)$ may need to be appropriately scaled in order to avoid chattering.

## Neural Network Model for MNIST

```
import torch.nn as nn
import torch.nn.functional as F
class MNIST_model(nn.Module):
    def __init__(self):
        super(MNIST_model, self).__init__()

        # 28 × 28 × 1 ⟹ 26 × 26 × 32
        self.conv1 = nn.Conv2d(in_channels=1, out_channels=32, kernel_size=3)
        self.d1 = nn.Linear(26 * 26 * 32, 128)
        self.d2 = nn.Linear(128, 10)

    def forward(self, x):
        # 32 × 1 × 28 × 28 ⟹ 32 × 32 × 26 × 26
        x = self.conv1(x)
        x = F.relu(x)

        # flatten ⟹ 32 × (32 × 26 × 26)
        x = x.flatten(start_dim = 1)

        # 32 × (32 × 26 × 26) ⟹ 32 × 128
        x = self.d1(x)
        x = F.relu(x)

        # logits ⟹ 32 × 10
        logits = self.d2(x)
        out = F.softmax(logits, dim=1)
        return out
```

## Neural Network Model for CIFAR10

```
import torch.nn as nn
import torch.nn.functional as F

class CIFAR10Net(nn.Module):
    def __init__(self):
        super().__init__()
        self.conv1 = nn.Conv2d(3, 6, 5)
        self.pool = nn.MaxPool2d(2, 2)
        self.conv2 = nn.Conv2d(6, 16, 5)
        self.fc1 = nn.Linear(16 * 5 * 5, 120)
        self.fc2 = nn.Linear(120, 84)
        self.fc3 = nn.Linear(84, 10)

    def forward(self, x):
        x = self.pool(F.relu(self.conv1(x)))
        x = self.pool(F.relu(self.conv2(x)))
        x = torch.flatten(x, 1) # flatten all dimensions except batch
        x = F.relu(self.fc1(x))
        x = F.relu(self.fc2(x))
        x = self.fc3(x)
        return x
```
